# Supplementary material for: A Minimal Formulation of Session Types: The Sessions of Trios in Concert
Source: arXiv:2301.05301 source file (2025-05-12)
Supplement: Supplementary file 4 [file appendix-mst-ho-aux.tex]

\section{Auxiliary Results}
\begin{remark}
	\label{r:polyadic-rules}
	We derive polyadic rules for typing \HOp as an expected extension of
	\HO typing rules:

  \begin{prooftree}
    \AxiomC{}
    \LeftLabel{\scriptsize PolyVar}
    \UnaryInfC{$\Gamma, \wtd x : \wtd U_x;\wtd y :
                  \wtd U_y; \es \proves
                  \wtd x \wtd y :\wtd U_x \wtd U_y$}
  \end{prooftree}

  \begin{prooftree}
  	\AxiomC{}
  	\LeftLabel{\scriptsize PolySess}
  	\UnaryInfC{$\Gamma;\es;\wtd u:\wtd S
  				\proves \wtd u \hastype \wtd S$}
  \end{prooftree}

	\begin{prooftree}
		\AxiomC{$\Gamma;\Lambda_1;\Delta \cat u:S \proves P \hastype \Proc$}
		\AxiomC{$\Gamma;\Lambda_2;\es \proves \wtd x \hastype \wtd U$}
		%\AxiomC{$u \in \Delta$}
		\LeftLabel{\scriptsize PolyRcv}		\BinaryInfC{$\Gamma \setminus \wtd x;\Lambda_1 \setminus \Lambda_2; \Delta \cat
		u:\btinp{\wtd U}S
		\proves
		\binp{u}{\wtd x}P \hastype \Proc
		$}
	\end{prooftree}

	\begin{prooftree}
		\AxiomC{$u:S \in \Delta$} 
		\AxiomC{$\Gamma;\Lambda_1;\Delta \proves P$}
		\AxiomC{$\Gamma;\Lambda_2;\es \proves
						\wtd x \hastype \wtd U$}
		\LeftLabel{\scriptsize PolySend}
		\TrinaryInfC{$\Gamma;\Lambda_1 \cat \Lambda_2;
							(\Delta \setminus u:S) \cat
							u:\btout{\wtd U}S \proves
							\bout{u}{\wtd x}P$}
	\end{prooftree}
	\begin{prooftree}
		\AxiomC{$\leadsto \in \{\multimap,\rightarrow \}$}
		\AxiomC{$\Gamma;\Lambda;\Delta_1 \proves V \hastype \wtd C \leadsto \diamond$}
		\AxiomC{$\Gamma;\es;\Delta_2 \proves \wtd u \hastype \wtd C$}
		\LeftLabel{\scriptsize PolyApp}
		\TrinaryInfC{$\Gamma;\Lambda;\Delta_1 \cat \Delta_2 \proves
						\appl{V}{\wtd u}$}
	\end{prooftree}

	\begin{prooftree}
		\AxiomC{$\Gamma;\Lambda;\Delta_1 \proves P \hastype \Proc$}
		\AxiomC{$\Gamma;\es;\Delta_2 \proves \wtd x \hastype \wtd C$}
		\LeftLabel{\scriptsize PolyAbs}
		\BinaryInfC{$\Gamma \setminus \wtd x;\Lambda;\Delta_1 \setminus \Delta_2 \proves \abs{\wtd x}{P} \hastype \lhot{\wtd C}$}
	\end{prooftree}

	\begin{prooftree}
		\AxiomC{$\Gamma \cat \wtd a : \wtd {\chtype{U}};\Lambda;\Delta \proves
					P$}
		%\AxiomC{$\wtd S_1 \ \dualof \ \wtd S_2$}
		\LeftLabel{\scriptsize PolyRes}
		\UnaryInfC{$\Gamma;\Lambda;\Delta \proves
						\news{\wtd a}{P}$}
	\end{prooftree}

	\begin{prooftree}
		\AxiomC{$\Gamma;\Lambda;\Delta \cat \wtd s:\wtd S_1
					\cat \dual{\wtd s}:\wtd S_2 \proves
					P$}
		\AxiomC{$\wtd S_1 \ \dualof \ \wtd S_2$}
		\LeftLabel{\scriptsize PolyResS}
		\BinaryInfC{$\Gamma;\Lambda;\Delta \proves
						\news{\wtd s}{P}$}
	\end{prooftree}


\end{remark}

\begin{lemm}[Substitution Lemma~\cite{DBLP:conf/esop/KouzapasPY16}]
  \label{lem:subst}
  $\Gamma;\Lambda;\Delta \cat x : S \proves P \hastype \Proc$
  and $u \notin \text{dom}(\Gamma,\Lambda,\Delta)$ implies
  $\Gamma;\Lambda;\Delta \cat u : S \proves P \subst{u}{x} \hastype \Proc$.
\end{lemm}

\begin{lemm}[Shared environment weakening]
	\label{lem:weaken}
	If $\Gamma;\Lambda;\Delta \proves P \hastype \Proc$
	then
	$\Gamma \cat x:\shot{C};\Lambda;\Delta \proves P \hastype \Proc$ and
	$\Gamma \cat u:\chtype{U};\Lambda;\Delta \proves P \hastype \Proc$.
\end{lemm}

\begin{lemm}[Shared environment strengthening]
	\label{lem:strength}
	\begin{itemize}
	\item	If $\Gamma;\Lambda;\Delta \proves P \hastype \Proc$ and
	$x \notin \fv{P}$ then $\Gamma \setminus x;\Lambda;\Delta \proves P \hastype \Proc$.
	\item If $\Gamma;\Lambda;\Delta \proves P \hastype \Proc$ and
	$u \notin \fn{P}$ then $\Gamma \setminus u;\Lambda;\Delta \proves P \hastype \Proc$.
	\end{itemize}
\end{lemm}
